# Supplementary material for: BlockGC: A Joint Learning Framework for Account Identity Inference on Blockchain with Graph Contrast
Source: arXiv:2112.03659 source file (2021-12-07)
Supplement: Supplementary file 1 [file appendix.pdf]

# Subgraph Contrastive Link Representation Learning (Appendix)

**Anonymous authors**

## Appendix

### A. Data Details

In citation network datasets — Cora, Citeseer and Pubmed (Sen et al. 2008) — nodes represent papers with corresponding bag-of-words features, and edges represent citation relationships between papers.

**Facebook:** a page-page web graph of verified Facebook sites. Nodes represent official Facebook pages, and links are mutual likes between sites. Node features are extracted from the site descriptions created by the page owners to summarize the purpose of the site.

**Github:** a large social network where nodes are GitHub developers who have starred at least 10 repositories and edges are mutual follower relationships between them. Node features are extracted based on the location, repositories starred, employer and e-mail address.

For the two large datasets, their original features are not aligned. We create tagged documents from feature hash and further process them into 128-dimensional initial features by Doc2Vec algorithm. Both of the Facebook and Github datasets are available online [1].

### B. Data Preparation Details

We sample the same number of positive and negative links from the subgraph induced by nodes of top 60% largest degree values for each dataset $\{$Cora, Citeseer, Pubmed, Facebook, Github$\}$, with the proportion of $\{40\%, 40\%, 10\%, 10\%, 20\%\}$. We repeat 10-fold cross validation for 5 times, with the random seed of $\{987, 123, 4, 636, 723\}$.

### C. Parameter Configuration Details

In the experiments, we set the default GNN encoder of SCLRL to graph isomorphism network (GIN) (Xu et al. 2018) which is a recent GNN architecture provides a better inductive bias for graph level applications than GCN, as illustrated in Figure 1. GIN is a 2-layers graph convolutional network with jumping connection. Following each linear layer is a ReLU activation function. We return batch-wise graph-level representations by sum pooling. We set the dimension of graph convolutional layers to 64. We use early stopping with a patience of 20. We set the initial learning rate to $10^{-2}$, and use learning rate decay with a decay factor of 0.1 and a patience of 15. The batch size is set to 128. We choose the number of GCN layers, the C parameter of the SVM, and the number of estimators in RF from $\{2, 3\}$, $\{10^{-3}, 10^{-2}, \cdots, 10^{2}, 10^{3}\}$, $\{100, 200, 500, 1000\}$, respectively.

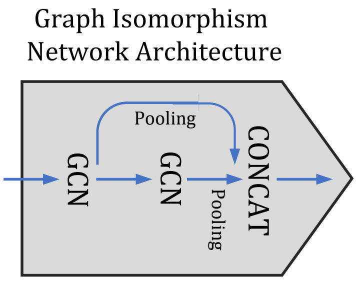


Figure 1: Illustration of graph isomorphism network.

For whole-graph embedding methods, we set the embedding dimension to 128. For Graph2Vec, we set the number of epochs to 500, and use the default setting for other parameters.

For random walks, we set the length of walks to 30, the number of walks to 200, and the context size to 10. For Node2Vec, we set the return parameter $p$ and in-out parameter $q$ to 4 and 1, respectively.

For graph auto-encoders, we use the default setting in (Kipf and Welling 2016). Specifically, we set the number of GCN layers, the number of epochs and learning rate to 2, 200 and $10^{-2}$, respectively. We use a 32-dim hidden layer and 16-dim latent variables in all experiments.

For SEAL, we choose the number of hops from $\{1, 2\}$. Note that we set the number of sampled neighborhs in hop 1 and hop 2 $(K_1, K_2)$ for each node to 3 when $K_1, K_2 = \text{ours}$, and $K_1, K_2 = \text{all}$ means that we sample all neighborhs in hop 1 and hop 2. For other parameters, we use the default setting following (Zhang and Chen 2018).

We refer to the following websites when implementing above models:

- **Graph Kernels**: https://github.com/ysig/GraKeL

Copyright © 2022, Association for the Advancement of Artificial Intelligence (www.aaai.org). All rights reserved.

[1] http://snap.stanford.edu/data/

- **Graph Embeddings**: https://github.com/benedekrozemberczki/karateclub
- **Random Walks**: https://github.com/shenweichen/GraphEmbedding
- **Graph Auto-Encoder**: https://github.com/zfjsail/gae-pytorch
- **SEAL**: https://github.com/muhanzhang/SEAL

## D. Versions of Package and Software

Regarding package and software versions, we install CUDA 10.2 and cuDNN 8.0. PyTorch 1.6.0 and Pytorch-Geometric 1.7.2 with Python 3.7.10 are used. Note that all the experiments are running at Ubuntu 18.04.5 LTS with the Intel(R) Xeon(R) Gold 5218R CPU @ 2.10GHz, and NVIDIA Tesla V100S GPU (with 40GB memory each).

## E. Effect of Subgraph Size

We further investigate the impact of subgraph size in our framework on large-scale datasets. We first fix $h = 1$ and adjust $K_1$ from 2 to 10, and evaluate the results shown in Figure 2. We observe that our model obtains best result on Facebook dataset when $K_1 = 3$, which is similar to that in citation networks. For Github dataset, our model performs better with a larger $K_1$ ($> 8$). Note that there is an interesting finding, when $K_1 = 3$, our 1-hop SCLRL achieves global optimality on three citation networks and Facebook dataset, while achieves local optimality on Github dataset which has a relative larger scale.

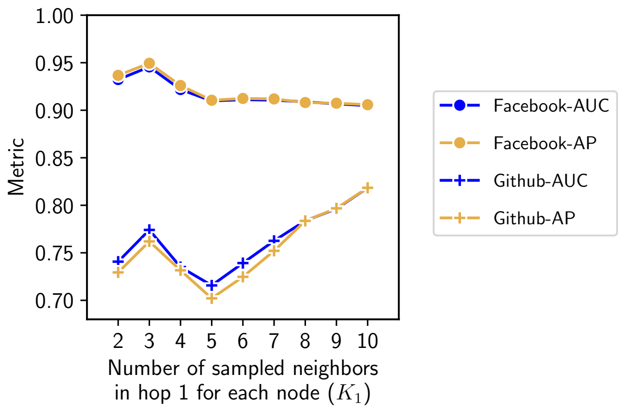


Figure 2: Performance versus subgraph size in large-scale datasets.

## F. Pseudocode

The pseudocode of our SCLRL is presented in Algorithm 1.

Algorithm 1: Subgraph Contrastive Link Representation Learning algorithm.

**Input:** Graph $\mathcal{G} = (\mathcal{V}, \mathcal{E}, \mathbf{X})$, hop $h$, topK $\{K\}$, target links $L_{emb}$, batch size $n$, augmentor $t_1$ and $t_2$, encoder $f_\theta$, projection head $f_\phi$;

Sample slci-subgraphs from graph: $\mathcal{D} = \mathsf{subgraphSampler}(\mathcal{G}, h, \{K\}, L_{emb})$ ;

`// compute encodings:`

**for** *sampled batch* $\{g_i\}_{i=1}^n \in \mathcal{D}$ **do**

  **for** $i = 1$ *to* $n$ **do**

    $\hat{g}_i^1 = (\hat{\mathbf{A}}_i^1, \hat{\mathbf{X}}_i^1) \leftarrow t_1(g_i)$ ; `// first view`

    $\mathbf{h}_i^1 \leftarrow f_\theta(\hat{\mathbf{X}}_i^1, \hat{\mathbf{A}}_i^1)$ ; `// graph rep.`

    $\mathbf{z}_i^1 \leftarrow f_\phi(\mathbf{h}_i^1)$ ; `// projected graph rep.`

    $\hat{g}_i^2 = (\hat{\mathbf{A}}_i^2, \hat{\mathbf{X}}_i^2) \leftarrow t_2(g_i)$ ; `// second view`

    $\mathbf{h}_i^2 \leftarrow f_\theta(\hat{\mathbf{X}}_i^2, \hat{\mathbf{A}}_i^2)$ ; `// graph rep.`

    $\mathbf{z}_i^2 \leftarrow f_\phi(\mathbf{h}_i^2)$ ; `// projected graph rep.`

  `// compute loss:`

  **define** $\mathcal{L}_i = -\log \frac{e^{\mathrm{s}\left(\mathbf{z}_i^1, \mathbf{z}_i^2\right)/\tau}}{\sum_{j=1, j\neq i}^n e^{\mathrm{s}\left(\mathbf{z}_i^1, \mathbf{z}_j^2\right)/\tau}}$

  $\mathcal{L} = \frac{1}{n}\sum_{i=1}^n \mathcal{L}_i$

  `// compute gradients:`

  Update encoder $f_\theta$ and $f_\phi$ to minimize $\mathcal{L}$

**return** *Encoder* $f_\theta$

# References

Kipf, T. N.; and Welling, M. 2016. Variational Graph Auto-Encoders. *NIPS Workshop on Bayesian Deep Learning*.

Sen, P.; Namata, G.; Bilgic, M.; Getoor, L.; Galligher, B.; and Eliassi-Rad, T. 2008. Collective classification in network data. *AI Magazine*, 29(3): 93–93.

Xu, K.; Hu, W.; Leskovec, J.; and Jegelka, S. 2018. How Powerful are Graph Neural Networks? In *Proceedings of the 6th International Conference on Learning Representations*.

Zhang, M.; and Chen, Y. 2018. Link prediction based on graph neural networks. In *Proceedings of the 32nd International Conference on Neural Information Processing Systems*, volume 31, 5165–5175.
